# Supplementary material for: An Analytical and AI-discovered Stable, Accurate, and Generalizable Subgrid-scale Closure for Geophysical Turbulence
Source: arXiv:2509.20365 ancillary file (2026-01-01)
Supplement: Supplementary file 1 [file PRL_GM_SI.pdf]

# Supplementary Information: An Analytical and AI-discovered Stable, Accurate, and Generalizable Subgrid-scale Closure for Geophysical Turbulence

Karan Jakhar,<sup>1,2</sup> Yifei Guan,<sup>1,3</sup> and Pedram Hassanzadeh<sup>4</sup>

<sup>1</sup>*Department of Geophysical Sciences, University of Chicago*

<sup>2</sup>*Department of Mechanical Engineering, Rice University*

<sup>3</sup>*Department of Mechanical Engineering, Union College*

<sup>4</sup>*Department of Geophysical Sciences and Committee on Computational and Applied Mathematics, University of Chicago\**

## I. INTER-SCALE ENERGY AND ENSTROPY TRANSFER

Figure S1 and Table S1 compliment Fig. 2 of the main manuscript by presenting spectra of the inte-scale fluxes of energy ( $P_\tau$ ) and enstrophy ( $P_Z$ ) computed from the FDNS data the closures used in this study. Fig. S1 and Table S1 confirm that NGM4 and NGM6 capture both the *sign* and the *magnitude* of the energy and enstrophy cascades across scales, whereas classical eddy-viscosity models remain strictly and overly diffusive.

## II. ENERGY AND ENSTROPY BALANCE

Figure S2 illustrates the ratios of FDNS energy ( $E$ ) and enstrophy ( $Z$ ) relative those of the DNS as a function of LES grid size. LES NGM4 and NGM6 closures are stable for LES with resolution retaining  $> 80\%$  of its DNS enstrophy.

## III. A POSTERIORI VALIDATION OF THE CLOSURES

We benchmark the LES against the ground-truth FDNS by evolving LES with each closure from identical random initial conditions. Fig. S3 compares the probability density function (PDF) of vorticity and confirms that LES with NGM4 and NGM6 closures capture the tails essential for predicting extremes. Figure S4 and Table S2 capture the bulk of energy and enstrophy, better than the eddy-viscosity closure baselines.

TABLE S1. *A priori* comparison of the ratio of inter-scale energy ( $P_\tau$ ) and enstrophy ( $P_Z$ ) transfers of various SGS closures to the FDNS for  $N_{\text{LES}} = 128$  (Cases 1-2) and  $N_{\text{LES}} = 512$  (Cases 3-4). Positive sign indicates diffusion ( $P_\tau, P_Z > 0$ ), while negative sign shows backscattering ( $P_\tau, P_Z < 0$ ). NGM4 and NGM6 effectively capture the magnitude and direction (including backscatter) of inter-scale transfers, unlike eddy-viscosity closures. NGM4 and NGM6 closely match  $P_Z$  ( $\approx P_Z^{\text{FDNS}}$ ) and achieve 0.6-0.8 times the  $P_\tau^{\text{FDNS}}$ , a significant improvement over eddy-viscosity closures, which can have energy transfer up to 100 times that of FDNS in some cases. The FDNS exhibits energy backscattering, also captured by NGMs (except NGM2, where  $P_\tau^{\text{NGM2}} = 0$ ), whereas eddy-viscosity closures are purely diffusive (as indicated by the negative sign of the ratio).

| Closure | $\langle P_\tau \rangle / \langle P_\tau^{\text{FDNS}} \rangle$ |         |        |        | $\langle P_Z \rangle / \langle P_Z^{\text{FDNS}} \rangle$ |        |        |        |
|---------|-----------------------------------------------------------------|---------|--------|--------|-----------------------------------------------------------|--------|--------|--------|
|         | Case 1                                                          | Case 2  | Case 3 | Case 4 | Case 1                                                    | Case 2 | Case 3 | Case 4 |
| FDNS    | 1                                                               | 1       | 1      | 1      | 1                                                         | 1      | 1      | 1      |
| NGM2    | 0                                                               | 0       | 0      | 0      | 0.97                                                      | 0.99   | 0.99   | 0.99   |
| NGM4    | 0.6                                                             | 0.59    | 0.69   | 0.58   | 0.97                                                      | 0.99   | 1.0    | 0.99   |
| NGM6    | 0.75                                                            | 0.74    | 0.85   | 0.74   | 0.97                                                      | 0.99   | 0.99   | 0.99   |
| Smag    | -45.73                                                          | -124.65 | -41.11 | -32.98 | -2.48                                                     | -5.15  | -2.35  | -2.72  |
| DSmag   | -23.72                                                          | -53.47  | -18.47 | -15.99 | -1.29                                                     | -2.21  | -1.06  | -1.32  |
| DLeith  | -6.29                                                           | -11.21  | -5.19  | -4.37  | -0.34                                                     | -0.46  | -0.3   | -0.36  |

\* pedramh@uchicago.edu

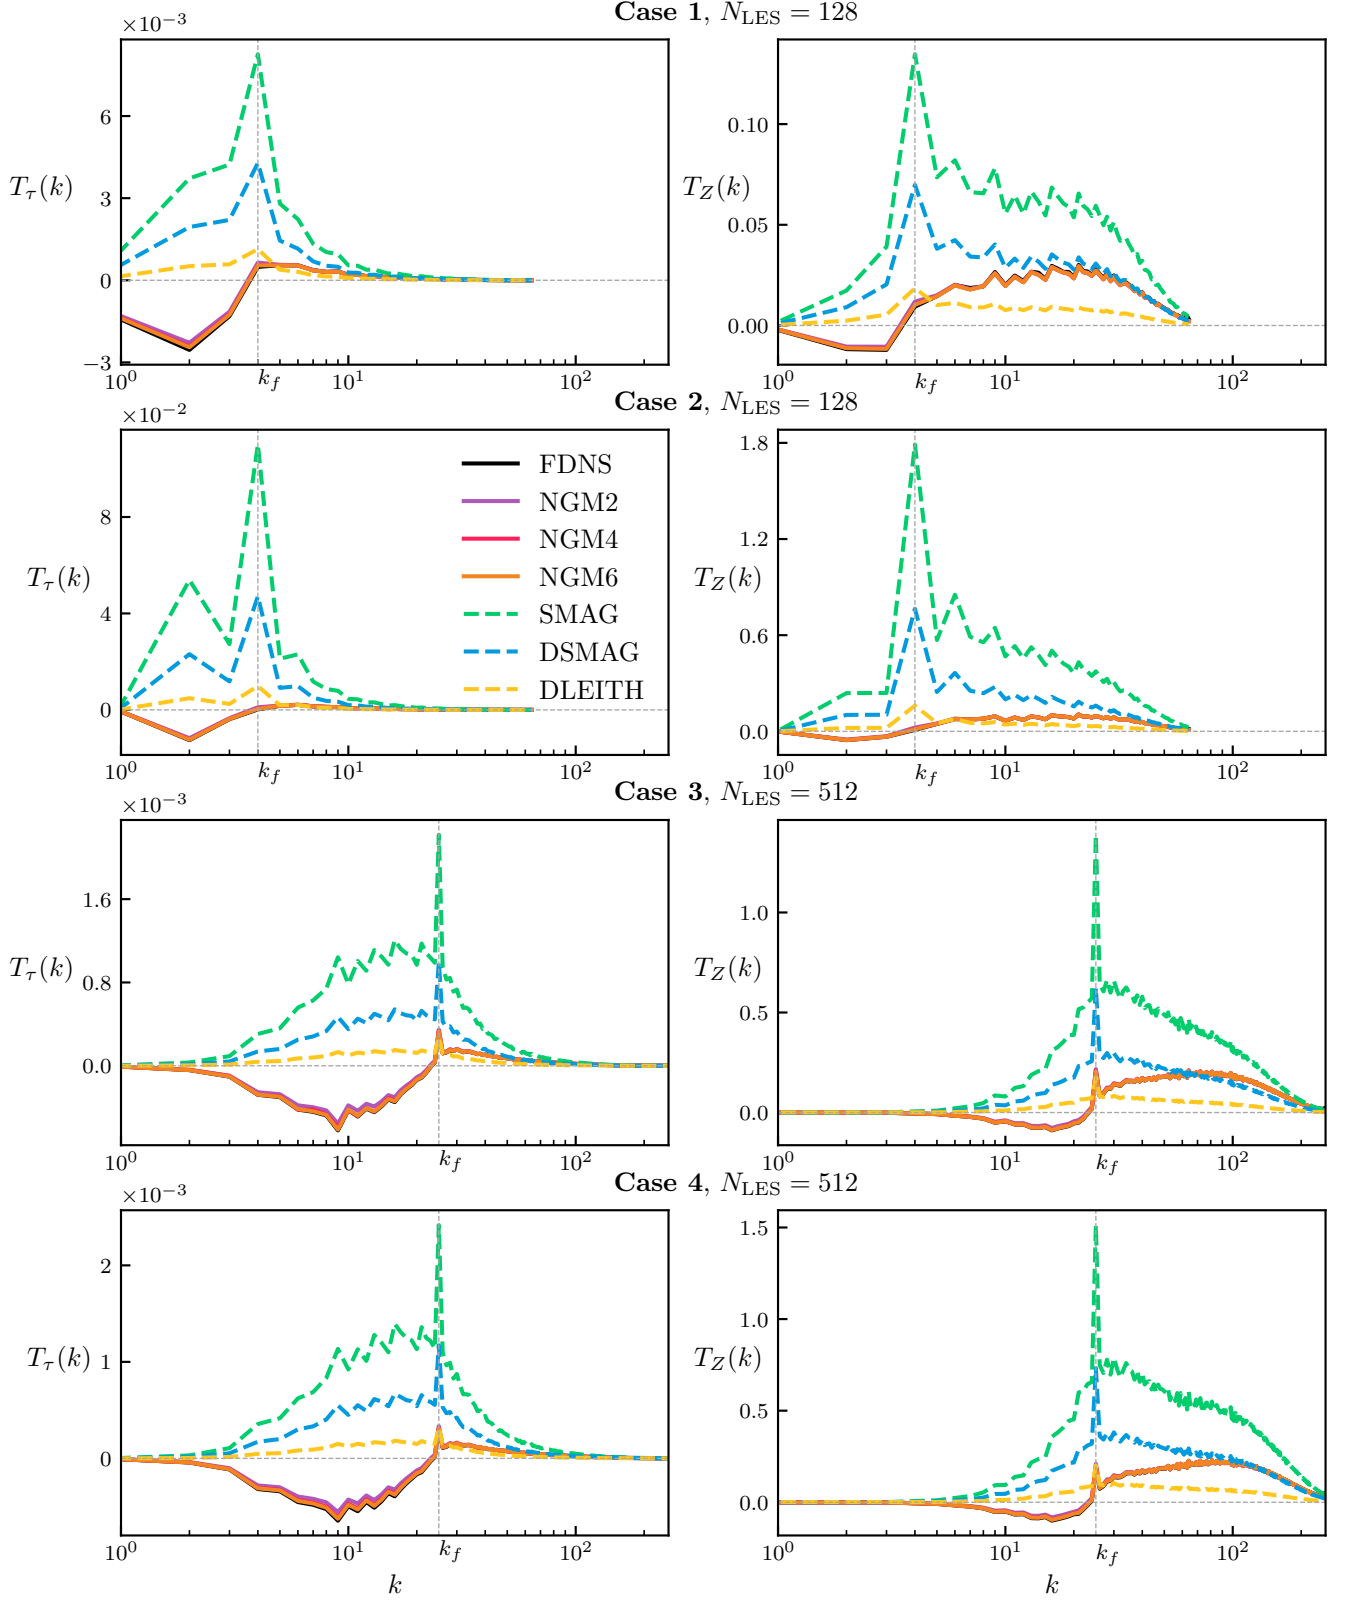

FIG. S1. Inter-scale energy  $T_\tau(k)$  and enstrophy transfer  $T_Z(k)$  spectra for four different cases. The first column shows the inter-scale energy transfer spectra, while the second column displays the inter-scale enstrophy transfer spectra. Cases 1-2 correspond to  $N_{\text{LES}} = 128$ , and Cases 3-4 correspond to  $N_{\text{LES}} = 512$ . Positive values (+) indicate diffusion ( $T_\tau(k), T_Z(k) > 0$ ), while negative values (-) indicate backscattering ( $T_\tau(k), T_Z(k) < 0$ ). NGMs (colored, solid lines) effectively capture the spectra across all scales, overlaying on top of FDNS spectra (black, solid line) and capturing both diffusion and backscatter accurately. In contrast, eddy-viscosity spectra (dashed solid lines) are diffusive across all wavenumbers.

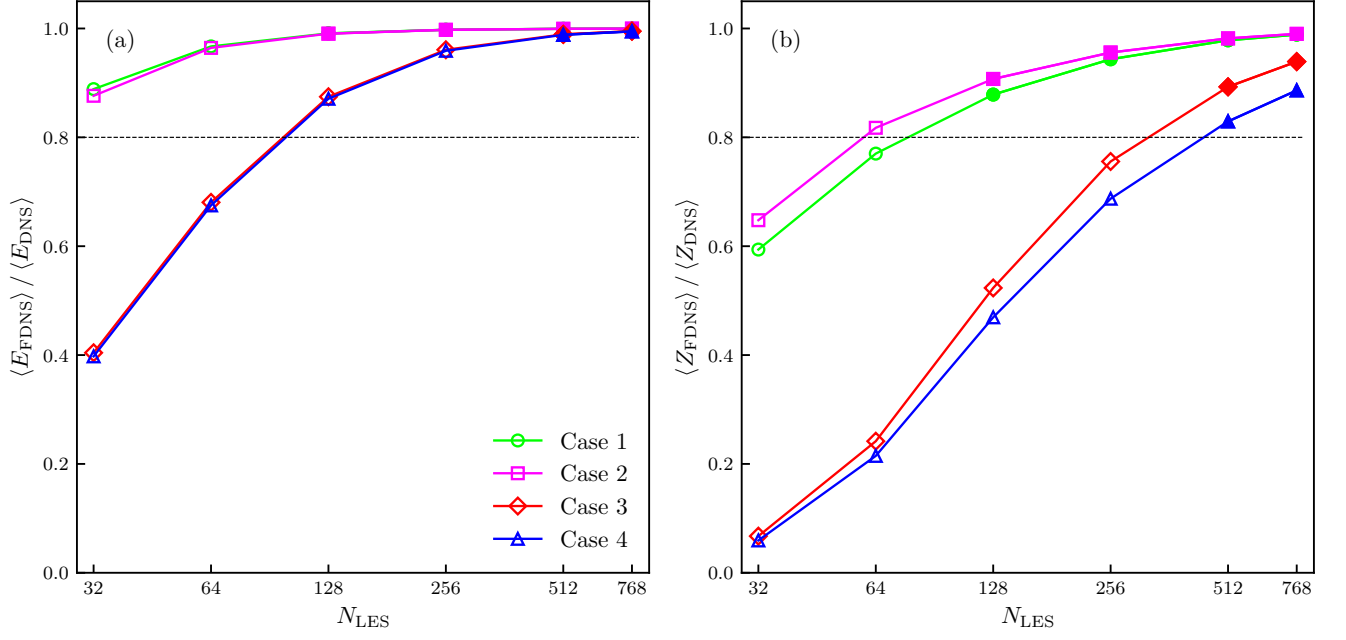

FIG. S2. (a) The ratio of FDNS kinetic energy to DNS kinetic energy, and (b) the ratio of FDNS enstrophy to DNS enstrophy. Note that the smallest  $N_{\text{LES}}$  for equation discovery is chosen such that the LES resolution resolves at least 80% of the DNS kinetic energy. LES NGM4 and NGM6 remain stable for  $N_{\text{LES}}$  values capturing more than 80% of the enstrophy (shown with filled symbols).

TABLE S2. *A posteriori* comparison of the ratio of energy ( $E$ ) and enstrophy ( $Z$ ) captured by various SGS closures to the FDNS for  $N_{\text{LES}} = 128$  (Cases 1-2) and  $N_{\text{LES}} = 512$  (Cases 3-4). LES with NGM4 and NGM6 can capture the bulk of energy within 2% of FDNS', and enstrophy within 5% of FDNS'. LES with Eddy-viscosity closures generally under-estimate both energy and enstrophy, with DLeith being the best-performing physics-based closure. LES with DLeith captures both energy and enstrophy within 5% of the FDNS, providing performance close to that of NGM4 and NGM6 in this metric.

| Closure | $\langle E_{\text{LES}} \rangle / \langle E_{\text{FDNS}} \rangle$ |        |        |        | $\langle Z_{\text{LES}} \rangle / \langle Z_{\text{FDNS}} \rangle$ |        |        |        |
|---------|--------------------------------------------------------------------|--------|--------|--------|--------------------------------------------------------------------|--------|--------|--------|
|         | Case 1                                                             | Case 2 | Case 3 | Case 4 | Case 1                                                             | Case 2 | Case 3 | Case 4 |
| FDNS    | 1                                                                  | 1      | 1      | 1      | 1                                                                  | 1      | 1      | 1      |
| NGM4    | 1.01                                                               | 1.00   | 1.02   | 1.01   | 1.05                                                               | 1.01   | 1.02   | 1.04   |
| NGM6    | 1.01                                                               | 1.01   | 1.02   | 1.01   | 1.04                                                               | 1.02   | 1.02   | 1.04   |
| SMAG    | 0.92                                                               | 0.83   | 0.81   | 0.78   | 0.88                                                               | 0.79   | 0.84   | 0.76   |
| DSMAG   | 0.93                                                               | 0.89   | 0.87   | 0.84   | 0.91                                                               | 0.86   | 0.9    | 0.82   |
| DLEITH  | 0.97                                                               | 0.96   | 0.95   | 0.93   | 1.00                                                               | 0.97   | 1.02   | 0.96   |

#### IV. GENERALIZED TAYLOR-SERIES EXPANSION OF THE SUBGRID-SCALE STRESS

We derive a generalized Taylor-series representation for the SGS stress that arises when the velocity field is convolved with a Gaussian filter [1, 2]. The resulting series can be written compactly as

$$\tau_{ij}^{\text{GM}} = \sum_{n=1}^{\infty} \frac{\Delta^{2n}}{12^n n!} \frac{\partial^n \bar{u}_i}{\partial x_{k_1} \cdots \partial x_{k_n}} \frac{\partial^n \bar{u}_j}{\partial x_{k_1} \cdots \partial x_{k_n}}, \quad (1)$$

where filter width,  $\Delta$ , is twice the LES grid size and repeated indices  $k_1, \dots, k_n$  are summed over according to the Einstein convention. The indices  $i$  and  $j$  remain free and designate the resolved-scale tensor components. Truncating the series after the first,  $n = 1$ , second,  $n = 2$ , and third,  $n = 3$ , terms yields the NGM2, NGM4, and NGM6, respectively.

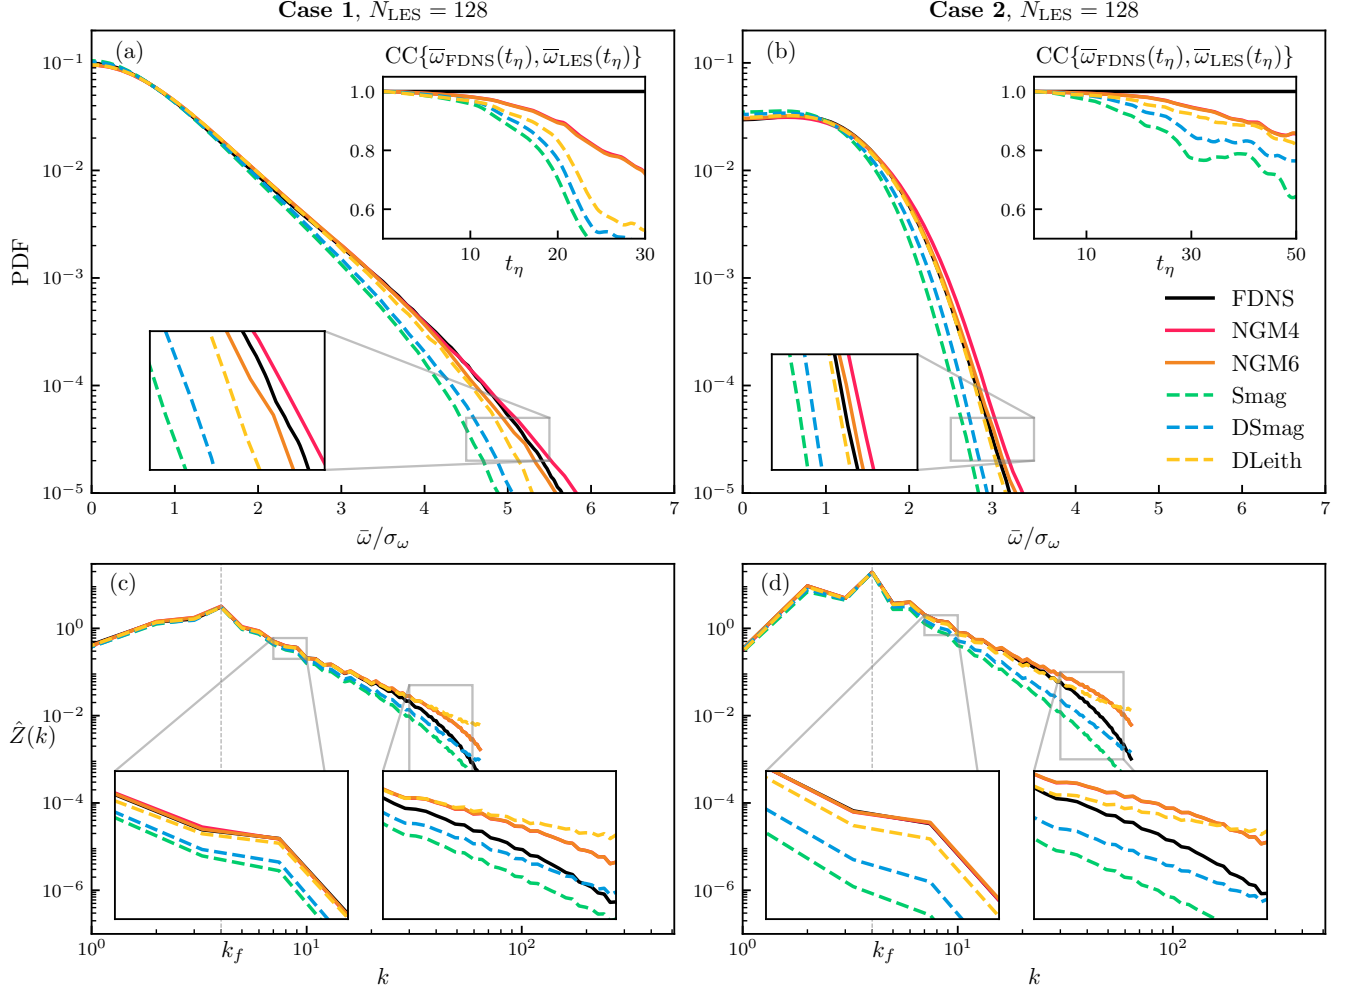

FIG. S3. Comparison of the *a posteriori* performance of different SGS closures for  $N_{\text{LES}} = 512$  (Cases 3-4). (a)-(b) The PDF of vorticity normalized by its standard deviation,  $\bar{\omega}/\sigma_{\omega}$ . The PDF of LES with NGM4 and NGM6 (solid red and orange lines) overlays on FDNS (solid black line), illustrating that LES with NGM4 and NGM6 can capture both the bulk and the tails of the PDF (as shown in the magnified inset of the tails), whereas LES with eddy-viscosity models (dashed lines) fail to do so, highlighting NGM4/6's capability to capture extreme events. The upper right insets of (a)-(b) further demonstrate NGM4/6's superiority over eddy-viscosity models in short-term forecasting by calculating the correlation coefficient (CC) between the vorticity of FDNS,  $\bar{\omega}_{\text{FDNS}}$ , and the SGS closures,  $\bar{\omega}_{\text{LES}}$ . The x-axis represents the eddy-turnover time,  $t_{\eta} = 1/\sqrt{\langle \bar{\omega}^2 \rangle}$ . All models start from the same initial condition, with LES with NGM4 and NGM6 maintaining a trajectory closer to FDNS than the LES with eddy-viscosity models. (c)-(d) Comparison of the enstrophy spectra,  $\hat{Z}(k)$ , of LES with different SGS closures. The insets magnifying the tails of the spectra do not clearly show the superior performance of any closure. However, the insets magnifying the spectra at lower wavenumbers clearly reveal that eddy-viscosity models struggle to capture the bulk of the enstrophy. This observation is also consistent for energy spectra (see Fig. S4). Table S2 further quantifies the bulk of energy and enstrophy captured by these SGS closures, confirming the aforementioned statement. It is important to note that NGM6 (solid orange line) overlays NGM4 (solid red line) in most panels, indicating similar performance with no significant advantage in transitioning from NGM4 to NGM6. A similar figure for  $N_{\text{LES}} = 512$  (Case 3-4) is shown in the manuscript.

## V. DECOMPOSITION OF THE SUBGRID-SCALE STRESS

We decompose the velocity into resolved and subgrid parts,  $u_i = \bar{u}_i + u'_i$ . Leonard [3] expressed  $\tau_{ij}$  as the sum of three stresses. Because two of Leonard's components are not Galilean-invariant [4], Germano [5] proposed the fully Galilean-invariant decomposition

$$\tau_{ij} = L_{ij} + C_{ij} + R_{ij}, \quad (2)$$

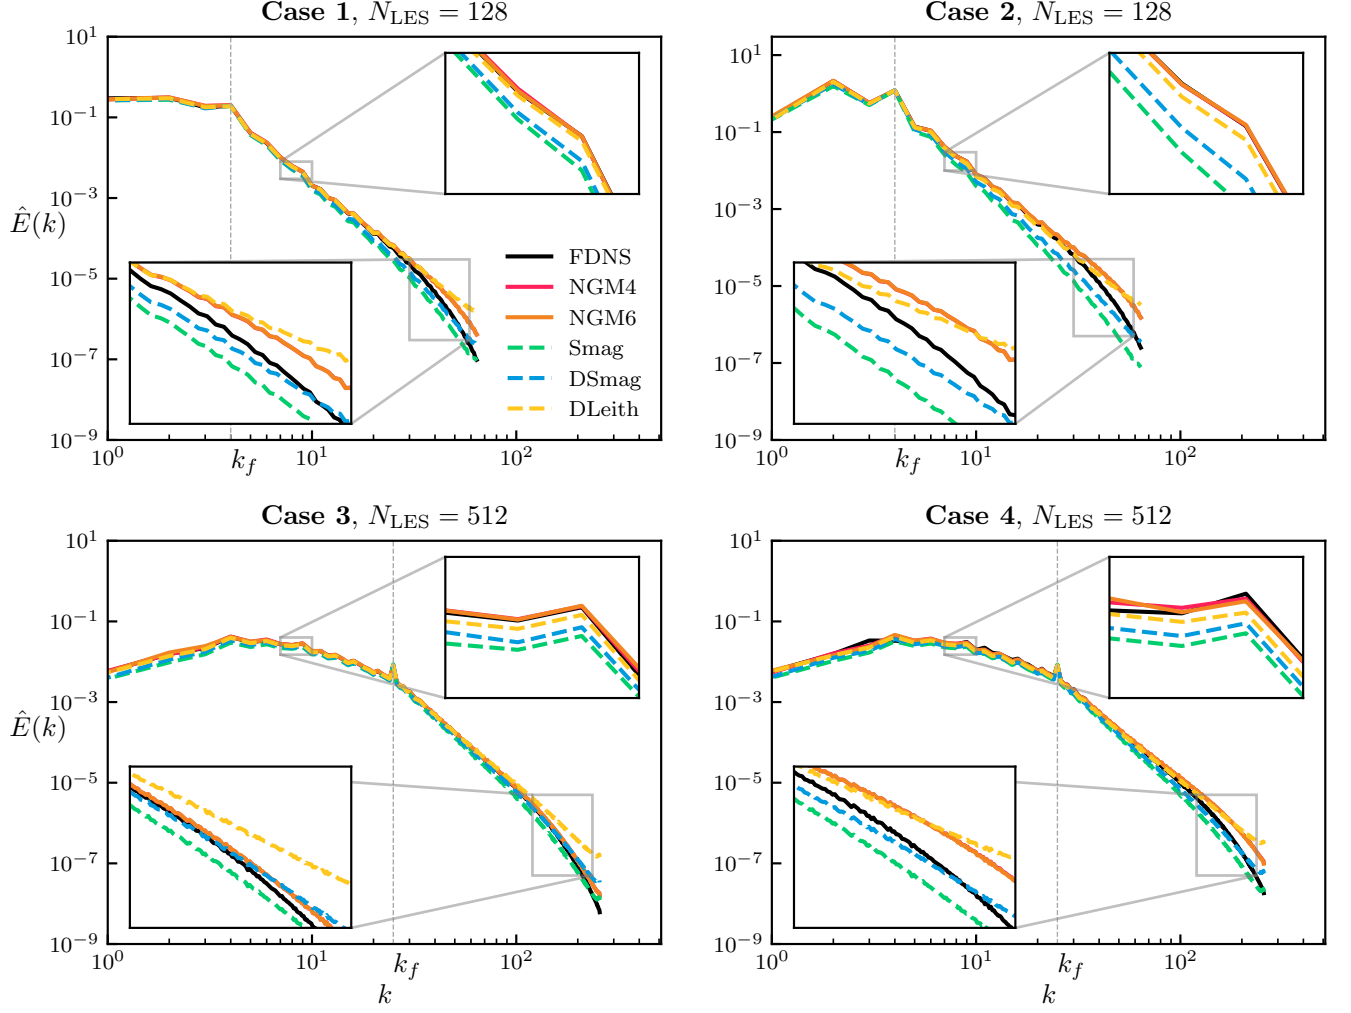

FIG. S4. Energy spectra of various SGS closures for  $N_{\text{LES}} = 128$  (Cases 1-2) and  $N_{\text{LES}} = 512$  (Cases 3-4). The inset at lower wavenumber shows that the NGM4 and NGM6 capture the bulk of the energy while eddy-viscosity models struggles. This observation is also consistent for enstrophy spectra (see Fig. S3). Table S2 further quantifies the bulk of energy and enstrophy captured by these SGS closures, confirming the aforementioned statement. It is important to note that NGM6 (solid orange line) overlays NGM4 (solid red line) in most panels, indicating similar performance with no significant advantage in transitioning from NGM4 to NGM6. The insets magnifying the tails of the spectra do not show the performance advantage of any closure.

with

$$L_{ij} = \overline{\bar{u}_i \bar{u}_j} - \bar{\bar{u}}_i \bar{\bar{u}}_j, \quad (\text{Leonard stress}), \quad (3a)$$

$$C_{ij} = \overline{\bar{u}_i u'_j} + \overline{u'_i \bar{u}_j} - \bar{\bar{u}}_i \overline{u'_j} - \overline{u'_i} \bar{\bar{u}}_j, \quad (\text{cross stress}), \quad (3b)$$

$$R_{ij} = \overline{u'_i u'_j} - \overline{u'_i} \overline{u'_j}, \quad (\text{Reynolds stress}). \quad (3c)$$

**Connection with NGMs:** While nonlinear gradient models (NGMs) are often described as Taylor series expansions of the subgrid-scale (SGS) term, in this work, we define the corresponding NGM for the Leonard, Cross and Reynolds stress. Applying the Taylor-series expansion of to each term in Eqs. (3a)-(3c) reveals [6]:

$$\text{NGM2: } L_{ij}^{\text{NGM2}} = \tau_{ij}^{\text{NGM2}}, \quad C_{ij}^{\text{NGM2}} = R_{ij}^{\text{NGM2}} = 0;$$

$$\text{NGM4: } \tau_{ij}^{\text{NGM4}} = L_{ij}^{\text{NGM4}} + C_{ij}^{\text{NGM4}}, \quad R_{ij}^{\text{NGM4}} = 0.$$

Thus NGM2 only includes the Leonard stress, whereas the NGM4 includes Leonard and cross stresses (while) still yielding zero Reynolds stress). NGM6 includes all three.

- 
- [1] P. Sagaut, *Large eddy simulation for incompressible flows: an introduction* (Springer Science & Business Media, 2006).
  - [2] K. Jakhar, Y. Guan, R. Mojgani, A. Chattopadhyay, and P. Hassanzadeh, Learning closed-form equations for subgrid-scale closures from high-fidelity data: Promises and challenges, *Journal of Advances in Modeling Earth Systems* **16**, e2023MS003874 (2024).
  - [3] A. Leonard, Energy cascade in large-eddy simulations of turbulent fluid flows, in *Advances in geophysics*, Vol. 18 (Elsevier, 1975) pp. 237–248.
  - [4] C. G. Speziale, Galilean invariance of subgrid-scale stress models in the large-eddy simulation of turbulence, *Journal of fluid mechanics* **156**, 55 (1985).
  - [5] M. Germano, A proposal for a redefinition of the turbulent stresses in the filtered Navier-Stokes equations, *The Physics of fluids* **29**, 2323 (1986).
  - [6] K. Jakhar, Sgstaylorx: Sgs taylor-series expansion (version 1.0) (2024).
